# Supplementary material for: Advantages of EEG phase patterns for the detection of gait intention in healthy and stroke subjects
Source: arXiv:1605.04533 ancillary file (2016-05-15)
Supplement: Supplementary file 1 [file Sburlea_Presentation_2.PDF]

# Supplementary materials

## Dataset 1

### Participants and experimental procedure

Ten volunteers (four females, mean age = 26.4 ± 4.8 years old) participated in the experiment. They were recruited from Bit&Brain Technologies in Zaragoza. All subjects were healthy without any known neurological anomalies and musculo-skeletal disorders. According to the Waterloo Footedness Questionnaire [1] seven out of ten subjects were right-footed. The experimental protocol was approved by the ethical committee of the HYPER project [1].

Participants were asked to perform the experiment in three sessions, with a week between sessions. The experimental protocol was the same during all three sessions.

Participants were standing on a wooden stage with their right leg pressing a footswitch inserted in the stage. The dimensions of the stage were 225.5 cm × 50 cm (length × width). Each trial was composed of two parts: relaxation and self-initiated movement. In the relaxation part that lasted ten seconds they were asked to stop moving, relax their muscles (to avoid possible contamination with muscular tension that could affect the outcome of the analysis) and to fixate their eyes on a point in the middle of the screen located at the end of the stage (to avoid contamination with ocular artifacts). The beginning of the movement part was marked by a fixation cross. The participants were previously informed that after the appearance of the fixation cross they can start walking whenever they want, but not earlier than 1.5 s[2]. The movement task was always initiated with the right leg. After each ten trials there were break intervals with a duration adjusted to the need of the participants. The breaks were marked by auditory cues. A phase consisted of ten trials and a break interval. A session had ten phases, enclosing a total of 100 trials.

### Data acquisition

EEG data were recorded using a TMSi REFA amplifier and a 30-channel EEG cap prepared for water based electrodes (from TMSi, Enschede, The Netherlands). The EEG sensors were located at Fp1, Fpz, Fp2, F7, F3, Fz, F4, F8, FC5, FC1, FC2, FC6, T7, C3, Cz, C4, T8, CP5, Cp1, Cp2, Cp6, P7, P3, Pz, P4, P8, POz, O1, Oz, O2, following the 10/10 international system, with the ground placed on the right wrist and two sensors on the ear lobes used for average linked ears reference. EMG data were recorded with the same amplifier using two bipolar Ag/AgCl electrodes on the top of soleus and tibialis anterior muscles of the right leg. These muscles were chosen as being consistently reported as one of the

[1]This project is part of the Spanish Ministry of Science Consolider Ingenio program, HYPER (Hybrid Neuroprosthetic and Neurorobotic Devices for Functional Compensation and Rehabilitation of Motor Disorders) - CSD2009-00067.

[2]The average timing between the fixation cross and the initiation of motion was 2.6 s with a standard deviation of 0.8 s.

first that activate in walking [2]. EEG and EMG electrodes impedance was kept below $5k\Omega$, and below $20k\Omega$, respectively. A footswitch located under the right sole was used to align the data to the movement onset (-0.5 seconds before the footswitch release). Shielded cables (TAS2, TMSi) were used to diminish the artifacts introduced by cable movements. EEG, EMG and footswitch signals were recorded at a sampling frequency of 256 Hz. The EEG signal was acquired with a power-line noise removal zero-phase Butterworth standard notch filter of fourth order at $48 - 52$ Hz and a zero-phase Butterworth bandpass filter of fourth order at $0.05 - 60$ Hz. The other signals were recorded without filtering. The amplifier was carried by the subjects in a backpack during the experiment.

## Dataset 2

### Participants and experimental procedure

Nine chronic stroke patients (three females, mean age = 59.7 years, SD = 11.3 years) participated in the experiment. They were recruited from the Clinic of University Rey Juan Carlos in Madrid, Spain. Demographic and clinical information of the participants is shown in Table 1.

Table 1: Demographic and clinical information of nine stroke patients.

| Patient number | Gender | Age (years) | Type of ictus | Affected brain hemisphere | Time since ictus (years) | Fugl-Meyer score | Particular brain condition |
|---|---|---|---|---|---|---|---|
| 1 | F | 52 | ischemic | left | 4.75 | 86 | no |
| 2 | F | 54 | ischemic | right | 16.5 | 66 | no |
| 3 | M | 41 | hemorrhagic | right | 13.66 | 62 | brain surgery |
| 4 | F | 69 | hemorrhagic | left | 2.33 | 81 | no |
| 5 | M | 76 | hemorrhagic | left | 1.75 | 73 | no |
| 6 | M | 67 | ischemic | left | 9.75 | 80 | no |
| 7 | M | 54 | ischemic | right | 4.66 | 69 | titanium plate |
| 8 | M | 71 | ischemic | left | 2 | 55 | no |
| 9 | M | 54 | ischemic | right | 1.42 | 72 | no |

All patients suffered hemispheric stroke (four on the right side and five on the left side). Three of the patients suffered a hemorrhagic stroke and six an ischemic stroke. According to the Waterloo Footedness Questionnaire [1] four out of nine subjects were right-footed. The Fugl-Meyer Assessment for Lower Extremity (FMA-LE), which consists of 43 items, with a maximum possible score of 86 points was administered to all patients. Each item was answered using a 3-point ordinal scale (0 = cannot perform, 1 = can partially perform, 2 = can fully perform). The assessment was completed by trained registered physical therapists. The experimental protocol was approved by the ethical committee of the HYPER project (approval number 12/104) [3] and all patients gave written consent before participating in the experiment.

[3] This project is part of the Spanish Ministry of Science Consolider Ingenio program, HYPER (Hybrid Neuroprosthetic and Neurorobotic Devices for Functional Compensation and Rehabilitation of Motor Disorders) - CSD2009-00067.

The experiment took place in the Motion Analysis, Ergonomics, Biomechanics and Motor Control Laboratory (LAMBECOM), Faculty of Health Sciences, Rey Juan Carlos University, Madrid, Spain. Patients performed the experiment in three sessions, with a week between sessions. The experimental protocol was the same during all three sessions. Each trial was composed of two parts: relaxation and movement. Both parts had variable time lengths according to the patient needs. The relaxation part started with an auditory cue that instructed the patients to relax and reduce movements. After approximately ten seconds another auditory cue instructed the patients to start walking whenever they want. Patients were previously instructed to wait a couple of seconds after hearing the second auditory cue. After every twenty trials there were break intervals with a duration adjusted to the need of the patients. A phase consisted of twenty trials and a break interval. A session had five phases, comprising a total of 100 trials.

### Data acquisition

EEG data were recorded using a TMSi Refa amplifier and a 30-channel EEG cap prepared for water based electrodes (from TMSi, Enschede, The Netherlands). The EEG sensors were located at Fp1, Fpz, Fp2, F7, F3, Fz, F4, F8, FC5, FC1, FC2, FC6, T7, C3, Cz, C4, T8, CP5, CP1, CP2, CP6, P7, P3, Pz, P4, P8, POz, O1, Oz, O2, following the 10/10 international system, with the ground placed on the right wrist and two sensors on the ear lobes used for average linked ears reference. Electromyographic (EMG) data were recorded with the same amplifier using two bipolar Ag/AgCl electrodes on the top of tibialis anterior muscles of the right and left legs. This muscle was chosen as being consistently reported as one of the first that activate in walking [2] of healthy subjects. EEG and EMG electrodes impedance was kept below $5K\Omega$, and below $20K\Omega$, respectively. Shielded cables (TAS2, TMSi) were used to diminish the artifacts introduced by cable movements. EEG and EMG signals were recorded at a sampling frequency of 256 Hz, without filtering. The amplifier was carried by the subjects in a backpack during the experiment.

The band-pass determination is always a compromise between reducing noise and artifact contamination, and preserving the desired information from the EMG signal [3, 4]. In their study, Luca et al. found that the information from the tibialis anterior muscle is observable in the frequency band between 20-200 Hz. After exploring different filters that would maximize the signal-to-noise ratio and allow a better detection of the movement onset, we found that most of the information was contained in the higher frequency bands therefore we used the Butterworth bandpass second order filter between 100-125 Hz. Next, the EMG data was Hilbert transformed and a threshold of 10% of the highest value from the averaged EMG power across trials was computed. The onset of motion was calculated as 100 ms before the considered threshold crossing.

# References


[1] Lorin J Elias, Mark P Bryden, and M Barbara Bulman-Fleming. Footedness is a better predictor than is handedness of emotional lateralization. *Neuropsychologia*, 36(1):37–43, 1998.

[2] DA Winter and HJ Yack. Emg profiles during normal human walking: stride-to-stride and inter-subject variability. *Electroencephalography and clinical neurophysiology*, 67(5):402–411, 1987.

[3] Gerhard Staude, Claus Flachenecker, Martin Daumer, and Werner Wolf. Onset detection in surface electromyographic signals: a systematic comparison of methods. *EURASIP Journal on Applied Signal Processing*, 2001(1):67–81, 2001.

[4] Carlo J De Luca, L Donald Gilmore, Mikhail Kuznetsov, and Serge H Roy. Filtering the surface emg signal: Movement artifact and baseline noise contamination. *Journal of biomechanics*, 43(8):1573–1579, 2010.
