# Supplementary material for: Advantages of EEG phase patterns for the detection of gait intention in healthy and stroke subjects
Source: arXiv:1605.04533 ancillary file (2016-05-15)
Supplement: Supplementary file 2 [file Sburlea_Presentation_1.PDF]

The table Healthy\_Subjects\_Data.csv with the following columns:

1. Subjects - an array with values between 1 and 10
2. Training session - an array with values between 1 and 3, corresponding to the session
3. Testing session - an array with values between 1 and 3, corresponding to the session  
 e. g. Training session = 1 and Testing session = 1 => intrasession condition  
 Testing session = 1 and Testing session = 2 => intersession condition
4. Model - an array with values between 1 and 3  
 '1' - Amplitude model  
 '2' - Phase model  
 '3' - Combined model (Amplitude+Phase)
5. Trial-based performance (percentage of correct trials)
6. Total number of trials
7. Number of correctly classified windows
8. Total number of windows
9. Empirical chance level for windows

#####

### The table Stroke\_Subjects\_Data.csv with the following columns:

1. Subjects - an array with values between 1 and 9
2. Training session - an array with values between 1 and 3, corresponding to the session
3. Testing session - an array with values between 1 and 3, corresponding to the session  
 e. g. Training session = 1 and Testing session = 1 => intrasession condition  
 Testing session = 1 and Testing session = 2 => intersession condition
4. Model - an array with values between 1 and 3  
 '1' - Amplitude model  
 '2' - Phase model  
 '3' - Combined model (Amplitude+Phase)
5. Trial-based performance (percentage of correct trials)
6. Total number of trials
7. Number of correctly classified windows
8. Total number of windows
9. Empirical chance level for windows

#####

### The table Healthy\_interSubject\_Data.csv with the following columns:

1. Subjects - an array with values between 1 and 10
2. Session - an array with values between 1 and 3, corresponding to the number of the session

ReadMe\_SuppMat.txt

3. Type of evaluation - an array with the values 1 and 2  
    '1' - Intrasubject  
    '2' - Intersubject
4. Model - an array with values of 3  
    '3' - Combined model (Amplitude+Phase)
5. Trial-based performance (percentage of correct trials)
6. Total number of trials
7. Number of correctly classified windows
8. Total number of windows
9. Empirical chance level for windows

#####

### The table Stroke\_interSubject\_Data.csv with the following columns:

1. Subjects - an array with values between 1 and 9
2. Session - an array with values between 1 and 3, corresponding to the number of the session
3. Type of evaluation - an array with the values 1 and 2  
    '1' - Intrasubject  
    '2' - Intersubject
4. Model - an array with values of 3  
    '3' - Combined model (Amplitude+Phase)
5. Trial-based performance (percentage of correct trials)
6. Total number of trials
7. Number of correctly classified windows
8. Total number of windows
9. Empirical chance level for windows
